# Supplementary material for: Floquet phonon lasing in multimode optomechanical systems
Source: arXiv:2101.10788 source file (2021-01-26)

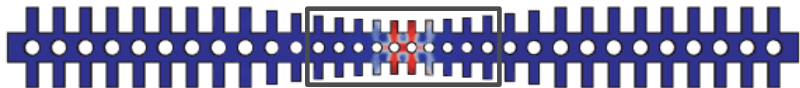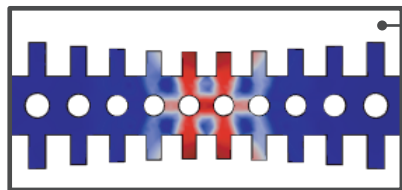

NOMINAL

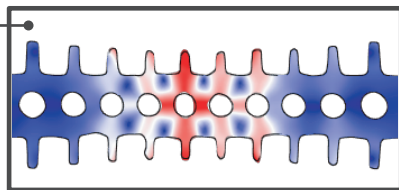

SEM RETRIEVED

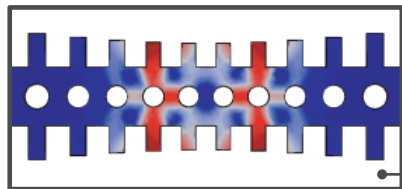

P1

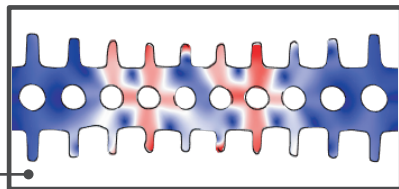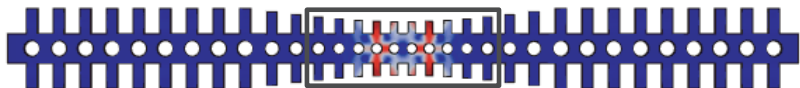

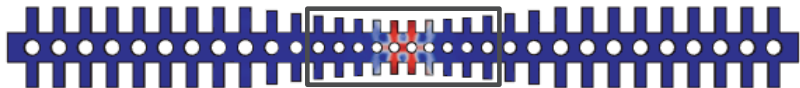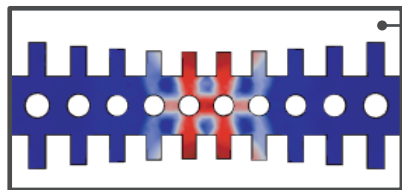

NOMINAL

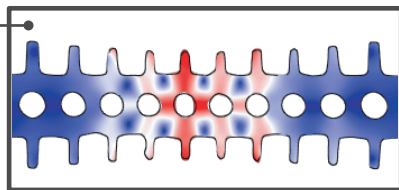

SEM RETRIEVED

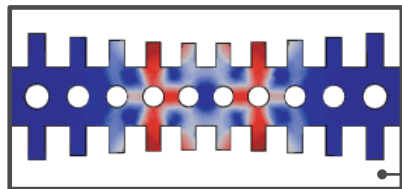

P1

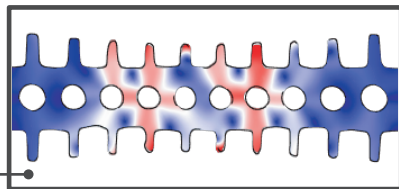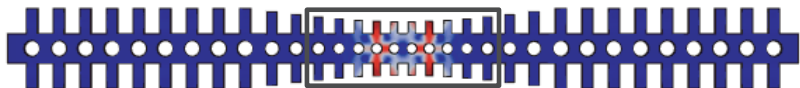

Supplement: Supplementary file 1 [file SUPP2.pdf]
